# Supplementary material for: Bayesian inference under model misspecification using transport-Lagrangian distances: an application to seismic inversion
Source: arXiv:2105.07027 source file (2021-05-14)
Supplement: Supplementary file 1 [file AppendixA.tex]

\clearpage

\section{Proof of theorem 3.1}

\begin{proof}

First, let us rewrite the $Z_k$ in more compact notation:
\begin{align}
    Z_k =   a_k + \lambda \sum_{j=1}^n \sum_{i=1}^n|| g(t_j) - f(t_i) ||^2  \sigma_{i,j}^k,
\end{align}
Where:
\begin{align*}
a_k     = \sum_{i=1}^{n}\sum_{j=1}^{n} \lambda ||x_i-y_j||^2 \sigma_{ij}^k .
\end{align*}
We note that the $f(t_i)$ are independent Gaussian r.v.s, each with a specific mean, but same variance, which allows us to state:
\begin{equation}
    X_l = \left( \frac{g(t_j) - f(t_i)}{\sigma} \right) ^2 \sim \chi^2_{1,\gamma=\mu_l^2}. \label{chisqX}
\end{equation}
Each $X_l$ is therefore a non-central\footnote{To completely specify a non-central chi-squared r.v. two parameters are needed: one indicating the degrees of freedom and another one indicating the non-centrality, which we call $\gamma$. This is equal to the sum of the squared means of each of the normal random variables being squared ad summed.} chi-squared r.v. with 1 degree of freedom and $\gamma=\mu_l^2$, where $\mu_l= \mu_{f(t_i)}-g(t_j)$. Although there are $n!$ possible values that $Z_k$ can take, $X_l$ can only take $n^2$ values, since there is only $n^2$ possible values that $|| g(t_j) - f(t_i) ||^2$ can assume. We can therefore express all the $Z_k$s as a linear system in $X_l$:
\begin{equation}
   \mathbf{Z} = \mathbf{A} + \sigma^2 \mathbf{ B X} \label{linearsys},
\end{equation}
where:
\begin{align*}
    \mathbf{Z} &= \left[Z_1, \dots, Z_{k} \right] \in \mathbb{R}_{\geq0}^{n! \times 1};\\
    \mathbf{A} &= \left[a_1, \dots, a_{k} \right] \in \mathbb{R}_{\geq0}^{n! \times 1}; \\
    \mathbf{X} &= \left[X_1, \dots, X_{n^2} \right] \in \mathbb{R}_{\geq0}^{n^2 \times 1}; \\
    \mathbf{B} &\in \{\{0,1 \}^{n! \times n^2} \text{s.t. }  B\mathbbm{1}^{n^2 \times 1} = n \mathbbm{1}^{n! \times 1} \}.
\end{align*}
B is a ``selector'' matrix which simply selects and sums the values of $X_l$ ($|| g(t_j) - f(t_i) || ^2$) that contribute to the $Z_k$ associated to permutation $\boldsymbol{\sigma}^k$. Because the B matrix only has $n$ entries equal to $1$ per row, each $\frac{Z_k-a_k}{\sigma^2}$ is then a non-central chi-squared r.v. with $n$ degrees of freedom and $\gamma$ specified as follows:
\begin{align}
    \frac{Z_k-a_k}{\sigma^2} \sim \chi_{n,
    \lambda}^2, \text{\,\,\,\, with: \,\,\,\, } \gamma = b_k[ \mu_1^2, \dots, \mu_{n^2}^2 ]^T, \label{chisqrv} 
\end{align}
where  $b_k$ is the k-th row of B.
At this point, the objective is to find an expression for the minimum $Z$ among the entries of $\mathbf{Z}$. 

\paragraph{\textbf{Calculating the CDF of Z}}

According to \cite{david2004order} and \cite{feller1957introduction} the CDF of the minimum Z of a generic set of random variables $\{Z_1, \dots Z_{n^2}\}$ (no independence or distributional assumptions) can be expressed by calculating the probability that \textit{at least} one of the $Z_k$ is less or equal to $z$. In particular:
\begin{align}
    &\mathbb{P}(Z \leq z) = \sum_{k=1}^{n!} (-1)^{k-1} S_k; \label{minim} \\
    & S_k = \sum_{\substack{r,q,w, \dots \\ r,q,w \dots \in \{1, 2, \dots n!\} \\\vert \{r,q, w,\dots \}\vert= k }} \mathbb{P}\left(Z_r \leq z, Z_q \leq z, \dots, Z_w \leq z  \right).
\end{align}
The term $S_k$ has to be interpreted as the sum of the joint CDFs of all subsets of cardinality $k$ of the $\{Z_1, \dots Z_{n!}\}$ r.v.s. \footnote{ Conceptually the formula just expresses the need to avoid ``double counting'' when dealing with events that ``overlap'' (dependency). For e.g. in the two dimensional case we would have:
\begin{align*}
    &\mathbb{P}(Z \leq z) = S_1 - S_2; \\
    & S_1 =  \mathbb{P}\left(Z_1 \leq z \right) + \mathbb{P}\left(Z_2 \leq z \right);  \\
    & S_2 =\mathbb{P}\left(Z_1\leq z, Z_2 \leq z \right).
\end{align*}
The probability of the minimum of two r.v.s being less or equal to $z$ is calculated as the sum of the probabilities of each of the two random variables being less than $z$ individually, minus (to avoid double counting) the probability of both of them being  less than $z$ simultaneously.} 

\paragraph{\textbf{Characterizing the asymptotic behavior of $Z_k$ }}
The problem therefore reduces to calculating the joint CDF of each subset of $Z_k$s needed to compute the above sum. While generally complex, we can obtain the joint CDFs of any subset of $\{Z_k\}_1^{n!}$ by exploiting their linear dependence to the $X_l$ and their particular covariance structure.

We have already stated that each $X_l$ is a non-central chi-squared r.v. with one degree of freedom. We have also already concluded that given the linearity of the relationship (\ref{linearsys}), the $\frac{Z_k-a_k}{\sigma^2}$ are non-central chi-squared random variables with $n$ degrees of freedom and parameter $\gamma$ as specified in (\ref{chisqrv}). Since a closed form expression for their CDF is not available, we  assume that $n > 100 $ (discretization points) and  approximate the distribution of the $\mathbf{B \cdot X}$ with a normal distribution (central limit theorem). In fact, even though the $\{ \chi^2_{1,\gamma=\mu_l^2} \}_1^{n^2}$ are not all independent from each other, each row of $\mathbf{B \cdot X}$ is a sum of $n$ independent $\chi^2_{1,\gamma=\mu_l^2}$ to which the central limit theorem can be applied. This statement can be justified as follows: recalling the definition
        \begin{equation}
            X_l = \left( \frac{g(t_j) - f(t_i)}{\sigma} \right) ^2 ,
        \end{equation} 
the particular nature of the assignment problem makes it such that a $Z_k$ will never be a sum of $X_l$s that originate from the same $f(t_i)$. Since the $f(t_i)$s are independent by construction, then we will always be dealing with a sum of independent random variables. 

With this assumption it becomes trivial to derive the distribution of any subset of $Z_k$ (linear combination of $X_l$, see (\ref{linearsys})). \\
Let us consider the subset containing the r.v. $\{Z_r,Z_q,\dots,Z_w
\}$.   Each of these subsets will  be distributed according to a multivariate Gaussian with mean and covariance matrix defined as:
\begin{align}
    \boldsymbol{\mu_{{r,q,\dots,w}}} &= 
        \begin{bmatrix}
        a_r \\
        a_q \\
        \dots \\
        a_w
        \end{bmatrix}
    + \sigma^2 \cdot
    \begin{bmatrix}
         \horzbar & b_r & \horzbar \\
         \horzbar & b_q & \horzbar\\
        &\dots &\\
         \horzbar & b_w & \horzbar
    \end{bmatrix}
    \cdot\mathbb{E}(\mathbf{X}), \\
    \mathbf{\Sigma}_{{r,q,\dots,w}} &= \sigma^4 
    \begin{bmatrix}
        \horzbar & b_r & \horzbar \\
         \horzbar & b_q & \horzbar\\
        & \dots &\\
         \horzbar & b_w & \horzbar
    \end{bmatrix}
    \cdot \mathbb{C}\text{ov}(\mathbf{X}) \cdot 
    \begin{bmatrix}
        \horzbar & b_r & \horzbar \\
         \horzbar & b_q & \horzbar\\
        &\dots &\\
         \horzbar & b_w & \horzbar
    \end{bmatrix}^T, 
\end{align}
where $a_k$ and $b_k$ are a generic row a $\mathbf{A}$ and $\mathbf{B}$ respectively. 

It remains to be specified what are the mean and covariance matrices for the vector  $\mathbf{X}$. As discussed before, the $X_l$ are non-central chi squared random variables. Therefore, referring to definitions in (\ref{chisqX}), we
have:
\begin{align*}
    \mathbb{E}(\mathbf{X}) &= 1 + [ \mu_1^2, \dots, \mu_{n^2}^2 ]^T. 
\end{align*}
For the covariance matrix, based on the independence-dependence structure of the $X_l$ (\ref{chisqX}) we have: 
\begin{align}
     \mathbb{C}\text{ov}(X_{l'},X_{l''}) = 0 \iff i_{l'} \neq i_{l''};   \\
     \mathbb{C}\text{ov}(X_{l'},X_{l''}) \neq 0  \iff i_{l'} = i_{l''}.  
\end{align}
In particular the non-zero entries of the matrix will be either on the diagonal ($i_{l'} = i_{l''}$ and $j_{l'} = j_{l''}$, which means $l'=l''$) or those $X_l$ that share the same $f(t_i)$, but whose mean has been off-set by a different constant ($g(t_j)$). While the value on the diagonal entries is simply the variance of each $X_l$, we report the value of the non-diagonal entries in appendix B only. The important aspect to remember is that, given the nature of the assignment problem, the non-diagonal-non-zero entries of
$\mathbb{C}\text{ov}(\mathbf{X})$ will be nullified by the zero entries of B in the product:
\begin{equation}
    B \cdot \mathbb{C}\text{ov}(\mathbf{X}) \cdot B^T,
\end{equation}
and thus we can impose, without error:
\begin{align*}
    \mathbb{C}\text{ov}(\mathbf{X}) &\triangleq \mathbb{I}_{n^2 \times n^2} \left(2 + 4 [ \mu_1^2, \dots, \mu_{n^2}^2 ]^T \right).
\end{align*}
Based the above discussion we are now able to propose an analytic expression for the CDF of $Z$ when $n$ is sufficiently large. Given:
\begin{equation}
    Z = \min \{Z_k\}_1^{n!},
\end{equation}
by calling $\boldsymbol{\Phi}_{\boldsymbol{\mu},\boldsymbol{\Sigma}}(\mathbf{z})$ the CDF of a multivariate normal distribution \footnote{
Before proceeding with the derivation of an expression for the PDF of $Z$, we note that a closed form expression for a multivariate normal CDF does not exist. At best, we can express $\boldsymbol{\Phi}_{\boldsymbol{\mu}_{{r,q,\dots,w}}, \mathbf{\Sigma}_{{r,q,\dots,w}}}(z)$ as:
\begin{equation}
    {\boldsymbol{\Phi}}_{\boldsymbol{\mu}_{r,q,\dots,w}, \mathbf{\Sigma}_{{r,q,\dots,w}}}(z) = \iint\dots \int_{-\infty}^z  \boldsymbol{\phi}(r,q, \dots,w)\, dr dq \dots dw,
\end{equation}
where $\boldsymbol{\phi}$ is the joint density function of a multivariate Gaussian with mean and covariance $\boldsymbol{\mu}_{{r,q,\dots,w}}, \mathbf{\Sigma}_{{r,q,\dots,w}}$.} with mean $\boldsymbol{\mu}$ and covariance $\boldsymbol{\Sigma}$, we have that:
\begin{align}
    &\mathbb{P}(Z \leq z) = \sum_{k=1}^{n!} (-1)^{k-1} S_k; \\
    & S_k = \sum_{\substack{r,q,\dots,w  \\ r,q,w \dots \in \{1, 2, \dots n!\} \\\vert \{r,q, \dots, w \}\vert= k }} \boldsymbol{\Phi}_{\boldsymbol{\mu}_{{r,q,\dots,w}}, \mathbf{\Sigma}_{{r,q,\dots,w}}}(z).
\end{align}

\paragraph{\textbf{PDF characterization from CDF}}

It is well know that in order to get the PDF of a random variable it is sufficient to derive its CDF. In our case it will be a total derivative w.r.t. $z$:
\begin{align}
    &\mathbb{P}(Z=z) =  \sum_{k=1}^{n!} (-1)^{k-1} S_k; \\
    & S_k = \sum_{\substack{r,q,\dots,w  \\ r,q,w \dots \in \{1, 2, \dots n!\} \\\vert \{r,q, \dots, w \}\vert= k }} \frac{d}{dz} \iint\dots \int_{-\infty}^z  \boldsymbol{\phi}(r,q, \dots,w)\, dr dq \dots dw. \label{integralZ}
\end{align}

The derivative of the integral in (\ref{integralZ}) is not a trivial one to calculate except in the case where k=1 \footnote{
We reinforce that the derivative (\ref{integralZ}) is not equivalent to :
\begin{equation}
    \frac{\partial^k}{\partial r \partial q \dots \partial w} \int^r\int^q\dots \int_{-\infty}^w  \boldsymbol{\phi}(r,q, \dots,w)\, dr dq \dots dw,
\end{equation}
which would easily resolve into a multivariate PDF evaluated a $z$.} We therefor proceed by induction and start with the case where $k=2$.
\begin{align}
    \mathbb{P}(Z=z) &= \frac{d}{dz} \mathbb{P}(Z_1\leq z) + \frac{d}{dz} \mathbb{P}(Z_2\leq z) + \frac{d}{dz} \mathbb{P}(Z_1\leq z, Z_2\leq z) = \\
    &=  \frac{d}{dz} \int_{-\infty}^z \phi_1(z_1) dz_1 +   \frac{d}{dz} \int_{-\infty}^z \phi_2(z_2) dz_2 +   \frac{d}{dz} \iint_{-\infty}^z \boldsymbol{\phi_{1,2}}(z_1,z_2) dz_1 dz_2.
\end{align}
The first two terms simply reduce to the respective PDFs ($\phi_1,\phi_2$) evaluated at $z$. The last term requires more analysis. We start by applying the definition of derivative:
\begin{align}
      \frac{d}{dz} \iint_{-\infty}^z \boldsymbol{\phi_{1,2}}(z_1,z_2) dz_1 dz_2 &= \lim_{h \to 0} \frac{1}{h} \left[ \iint_{-\infty}^{z+h} \boldsymbol{\phi_{1,2}}(z_1,z_2) dz_1 dz_2 -  \iint_{-\infty}^{z} \boldsymbol{\phi_{1,2}}(z_1,z_2) dz_1 dz_2 \right].
\end{align}
We split the first double integral (interval addition property):
\begin{dmath}
    \lim_{h \to 0} \frac{1}{h} \left[ \int_{-\infty}^{z+h}\int_{-\infty}^{z} \boldsymbol{\phi_{1,2}}(z_1,z_2) dz_1 dz_2 + \int_{-\infty}^{z+h}\int_{z}^{z+h} \boldsymbol{\phi_{1,2}}(z_1,z_2) dz_1 dz_2 - \iint_{-\infty}^{z} \boldsymbol{\phi_{1,2}}(z_1,z_2) dz_1 dz_2 \right], 
\end{dmath}
which in turn becomes:
\begin{dmath}
    \lim_{h \to 0} \frac{1}{h} \left[\cancel{ \iint_{-\infty}^{z} \boldsymbol{\phi_{1,2}}(z_1,z_2) dz_1 dz_2 }+\int_{z}^{z+h}\int_{-\infty}^{z} \boldsymbol{\phi_{1,2}}(z_1,z_2) dz_1 dz_2 + \int_{-\infty}^{z}\int_{z}^{z+h} \boldsymbol{\phi_{1,2}}(z_1,z_2) dz_1 dz_2 + \iint_{z}^{z+h} \boldsymbol{\phi_{1,2}}(z_1,z_2) dz_1 dz_2 -  \cancel{\iint_{-\infty}^{z} \boldsymbol{\phi_{1,2}}(z_1,z_2) dz_1 dz_2} \right].
\end{dmath}
The first and last term cancel out. We now expand the integrals in the $[z,z+h]$ interval using the trapezoidal rule (one interval of length $h$). The approximation is exact since we are working in the limit ($h\to0$). We have:
\begin{align}
    \lim_{h \to 0} \,\, &\frac{1}{h} \left[ h \left ( \frac{1}{2} \int_{-\infty}^{z} \boldsymbol{\phi_{1,2}}(z_1,z+h) dz_1 + \frac{1}{2} \int_{-\infty}^{z} \boldsymbol{\phi_{1,2}}(z_1,z) dz_1 \right ) \right] + \nonumber \\
    &+ \frac{1}{h} \left[ h \left ( \frac{1}{2} \int_{-\infty}^{z} \boldsymbol{\phi_{1,2}}(z+h,z_2) dz_2 + \frac{1}{2} \int_{-\infty}^{z} \boldsymbol{\phi_{1,2}}(z,z_2) dz_2 \right ) \right] + \label{integralsimplif} \\
    &+ \frac{1}{h} \left[ \frac{h^2}{4} \left ( \boldsymbol{\phi_{1,2}}(z,z) + \boldsymbol{\phi_{1,2}}(z,z+h) + \boldsymbol{\phi_{1,2}}(z+h,z) +\boldsymbol{\phi_{1,2}}(z+h,z+h)  \right ) \right] = \nonumber \\
    &= \int_{-\infty}^{z} \boldsymbol{\phi_{1,2}}(z_1,z) dz_1 + \int_{-\infty}^{z} \boldsymbol{\phi_{1,2}}(z,z_2) dz_2 + \cancelto{0}{h \boldsymbol{\phi_{1,2}}(z,z)}. \nonumber 
\end{align}
Given the fact that in each integral the joint distribution has one of the two variables fixed to being $z$, we can rewrite:
\begin{equation}
    \boldsymbol{\phi_{1,2}}(z_1,z) =  \phi_{1\vert 2 }(z_1) \phi_2(z), \,\,\,\,\,\,\,\,\, 
    \boldsymbol{\phi_{1,2}}(z,z_2) =  \phi_{2\vert 1 }(z_2) \phi_1(z),
\end{equation}
Substituting in (\ref{integralsimplif}):
\begin{equation}
    \int_{-\infty}^{z} \boldsymbol{\phi_{1,2}}(z_1,z) dz_1 +  \int_{-\infty}^{z} \boldsymbol{\phi_{1,2}}(z,z_2) dz_2 = \phi_2(z) \int_{-\infty}^{z} \phi_{1\vert 2 }(z_1) dz_1 + \phi_1(z) \int_{-\infty}^{z} \phi_{2\vert 1 }(z_2) dz_2
\end{equation}
and thus:
\begin{equation}
     \frac{d}{dz} \iint_{-\infty}^z \boldsymbol{\phi_{1,2}}(z_1,z_2) dz_1 dz_2 = \phi_1(z)\Phi_{2\vert1}(z) + \phi_2(z)\Phi_{1\vert2}(z).
\end{equation}
In the special case where $n=2$, this leads to:
\begin{equation}
    \mathbb{P}(Z=z)= \phi_1(z)+ \phi_2(z) - \phi_1(z)\Phi_{2\vert1}(z) - \phi_2(z)\Phi_{1\vert2}(z) \label{PDF2}
\end{equation}
The case where $k=3$ (see \ref{integralZ}) can be handled in the same way as $k=2$ and leads to a similar results (we omit calculations):
\begin{align}
    \frac{d}{dz} \iiint_{-\infty}^z \boldsymbol{\phi_{1,2,3}}(z_1,z_2,z_3) dz_1 dz_2 dz_3 &=  \phi_1\Phi_{2,3\vert1} + \phi_2\Phi_{1,3\vert2} + \phi_3\Phi_{1,2\vert3} + \\ 
    &+\boldsymbol{\phi}_{1,2}\Phi_{3\vert1,2} + \boldsymbol{\phi}_{1,3}\Phi_{2\vert1,3} +  \boldsymbol{\phi}_{2,3}\Phi_{1\vert2,3}  \nonumber
\end{align}
By induction we can therefore conclude that the derivative of the joint CDF of $k$ dependent normal r.v.s  can be built as follows:
\begin{itemize}
    \item Given a set $\{r,\dots,q,v,\dots,w\}$ of cardinality $k$;
    \item Consider all its possible subsets and associated complements e.g. $\{r,\dots,q\}$ and its complement $\{v,\dots,w\}$;
    \item The derivative of:
    \begin{align}
        \frac{d}{dz} \int\dots \iint_{-\infty}^z \dots \int  &\boldsymbol{\phi}(r,\dots, q,v, \dots,w)\, dr \dots dq,dv \dots dw = \\
        \sum_{\substack{ \{r,\dots,q\}; \{v,\dots,w\} \\ s.t.  \vert \{r,\dots,q\} \cup \{v,\dots,w\} \vert = k}} & \boldsymbol{\phi}_{r,\dots,q} \Phi_{v,\dots,w \vert r,\dots,q}
    \end{align}
    
\end{itemize}

\paragraph{\textbf{Conclusion}}Based on the above discussion we can therefore express the PDF of:
\begin{equation}
    Z = \min \{Z_k\}_1^{n!},
\end{equation}
as:
\begin{align}
    &\mathbb{P}(Z = z) = \sum_{k=1}^{n!} (-1)^{k-1} T_k \\
    & T_k = \sum_{\substack{r,q,\dots,v,w  \\ r,q,w \dots \in \{1, 2, \dots n!\} \\\vert \{r,q, \dots,v,w \}\vert= k }} \sum_{\substack{ \{r,\dots,q\}; \{v,\dots,w\} \\ s.t.  \vert \{r,\dots,q\} \cup \{v,\dots,w\} \vert = k}} \boldsymbol{\phi}_{r,\dots,q} \Phi_{v,\dots,w \vert r,\dots,q} \label{PDF}
\end{align} 
This expression is in fact generalizable to any set of r.v. (not necessarily normally distributed) as long as  their CDFs and PDFs are available (numerically or analytically). 
\end{proof}{}

We conclude this appendix by making some remarks on the interpretation of the above formula and compare it to the case where the $Z_k$ are independent. To facilitate the discussion we focus on the $n=2$ case, which allows an effective pictorial representation of the following expression (derived from (\ref{PDF2})):
\begin{align*}
    \mathbb{P}(\min \{ Z_1, Z_2 \} =z) &= \mathbb{P}(Z_1=z)+ \mathbb{P}(Z_2=z) + \\
    &- \mathbb{P}(Z_1=z)  \mathbb{P}(Z_2 \leq z\vert Z_1 =z)- \mathbb{P}(Z_2=z) \mathbb{P}(Z_1 \leq z \vert Z_2 =z)
\end{align*}
Once again this expression does not rely on the specific nature of the distribution of the single $Z_i$, but expresses a general principle represented in figure (\ref{fig:2dmin}). For a set of dependent and non-identically distributed random variables, we have that the probability of the minimum $Z$ being equal to a specific value $z$ is given by the sum of the probability of each r.v. being equal to $z$ minus (or plus) additional terms that take into account that when one of the r.v.s of the set is fixed to $z$ the others may not be less than $z$ or otherwise this would imply that $z$ is not the minimum. This concept is mathematically expressed, in the 2D case, through the product: $\mathbb{P}(Z_1=z)  \mathbb{P}(Z_2 \leq z\vert Z_1 =z)$   and $\mathbb{P}(Z_2=z)  \mathbb{P}(Z_1 \leq z\vert Z_2 =z)$.

\begin{figure}[h!]
    \centering
    \includegraphics{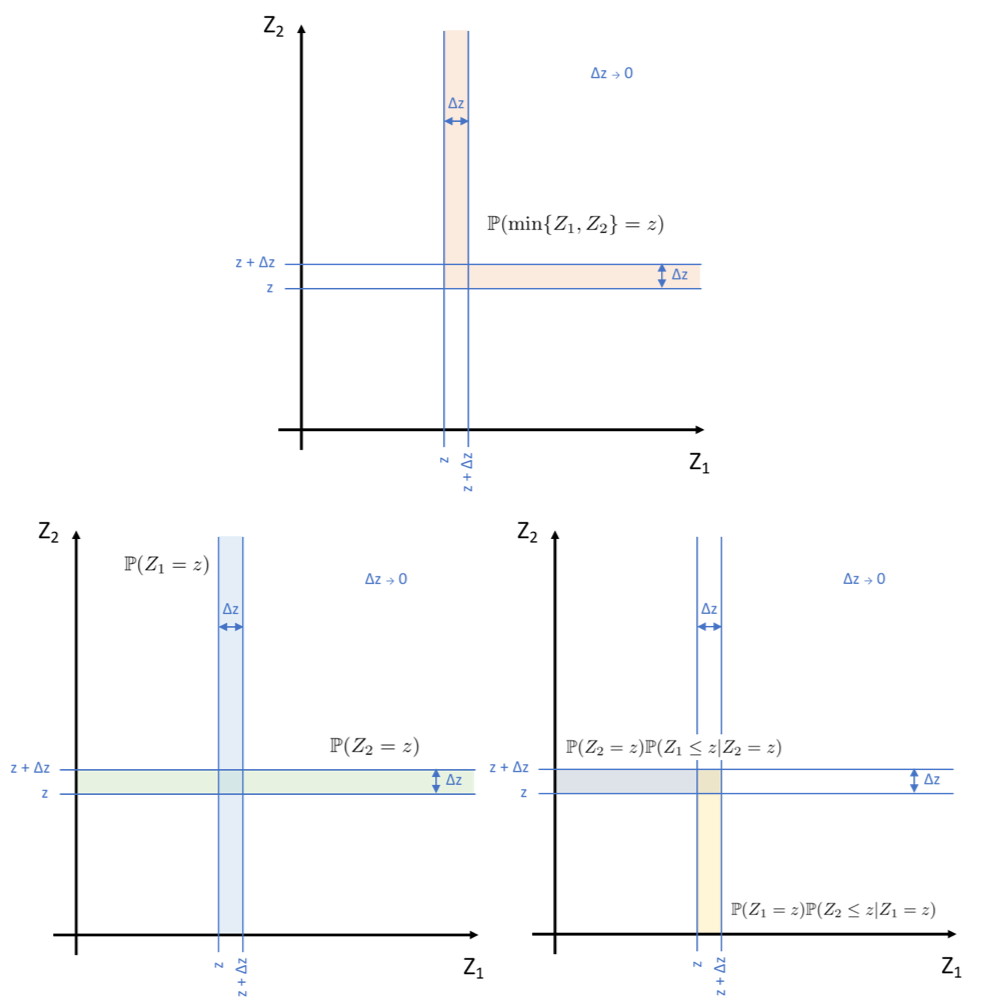}
    \caption{Construction of ${P}(\min \{ Z_1, Z_2 \} =z)$}
    \label{fig:2dmin}
\end{figure}{}
In the special case when the $Z_l$ are independent, then, by definition, $\mathbb{P}(Z_i \leq z \vert Z_j = z) = \mathbb{P}(Z_i \leq z)$ and in the 2-D case:
\begin{align}
    \mathbb{P}(\min \{ Z_1, Z_2 \} =z) &= \mathbb{P}(Z_1=z)+ \mathbb{P}(Z_2=z) \\
    &- \mathbb{P}(Z_1=z)  \mathbb{P}(Z_2 \leq z)+ \mathbb{P}(Z_2=z) \mathbb{P}(Z_1 \leq z )
\end{align}
This is consistent with the general formula for independent random variables:
\begin{align}
    \mathbb{P}(\min \{ Z_1, Z_2 \} =z) &= \frac{d}{dz} \left[1 - \left (1 - \mathbb{P}(Z_1 \leq z) ) (1- \mathbb{P}(Z_2 \leq z) \right ) \right] = \\
    &= (1 -\mathbb{P}(Z_1 \leq z))\mathbb{P}(Z_2=z) + (1 -\mathbb{P}(Z_2 \leq z))\mathbb{P}(Z_1=z) = \\
    &= \mathbb{P}(Z_1=z)+ \mathbb{P}(Z_2=z)  
    - \mathbb{P}(Z_1=z)  \mathbb{P}(Z_2 \leq z)+ \mathbb{P}(Z_2=z) \mathbb{P}(Z_1 \leq z ).
\end{align}
