# Supplementary material for: Bayesian inference under model misspecification using transport-Lagrangian distances: an application to seismic inversion
Source: arXiv:2105.07027 source file (2021-05-14)
Supplement: Supplementary file 2 [file AppendixB.tex]

\clearpage

\section{Covariance matrix for $X_l$}
The covariance matrix for the chi-squared non-central random variables is structured as follows:
\begin{equation}
\mathbb{C}\text{ov}(X_{l'},X_{l''})=
\begin{cases}
 \mathbb{V}\text{ar}(X_{l})= 2 + 4  \mu_l^2 &\iff l'=l'' \\
 0 &\iff l'\neq l'' \text{ and } i_{l'} \neq i_{l''} \\
 \beta &\iff l'\neq l'' \text{ and } i_{l'} = i_{l''}
\end{cases}
\end{equation}

The exact expression of $\beta$ is derived here below. Let:
\begin{align}
    X &=  \left( \frac{g(t_{j_{l'}}) - f(t_i)}{\sigma} \right) ^2 \\
    Y &=  \left( \frac{g(t_{j_{l''}})  - f(t_i)}{\sigma} \right) ^2 
\end{align}
Calling $\mathbb{E}(f(t_i))=\mu, a = g(t_{j_{l'}}), b= g(t_{j_{l''}})$,  we have:
\begin{align}
    \mathbb{E}(X)&= 1+ (a-\mu)^2    \\
    \mathbb{E}(Y)&= 1+ (b-\mu)^2    
\end{align}
consequently:
\begin{align}
    \mathbb{C}\text{ov}(X,Y)&= \beta = \mathbb{E}[(X-\mathbb{E}(X))(Y-\mathbb{E}(Y))] \\
    &= \mathbb{E} [\frac{a^2b^2}{\sigma^4}-\frac{2a^2b^2}{\sigma^2}+a^2b^2-\frac{2a^2bf}{\sigma^4}+\frac{2a^2bf}{\sigma^2}+\frac{2a^2b\mu}{\sigma^2}-2a^2b\mu+\frac{a^2f^2}{\sigma^4}-\frac{a^2f^2}{\sigma^2}-\frac{a^2\mu^2}{\sigma^2}+ \nonumber \\ &+ a^2\mu^2  -\frac{a^2}{\sigma^2}+a^2-\frac{2ab^2f}{\sigma^4}+\frac{2ab^2f}{\sigma^2}+\frac{2ab^2\mu}{\sigma^2}-2ab^2\mu+\frac{4abf^2}{\sigma^4}-\frac{8abf\mu}{\sigma^2}+4ab\mu^2 + \nonumber \\ &-\frac{2af^3}{\sigma^4}+\frac{2af^2\mu}{\sigma^2}+\frac{2af\mu^2}{\sigma^2}+\frac{2af}{\sigma^2}-2a\mu^3-2a\mu+\frac{b^2f^2}{\sigma^4}-\frac{b^2f^2}{\sigma^2}-\frac{b^2\mu^2}{\sigma^2}+b^2\mu^2-\frac{b^2}{\sigma^2}+ \nonumber \\
    &+b^2-\frac{2bf^3}{\sigma^4}+\frac{2bf^2\mu}{\sigma^2}+\frac{2bf\mu^2}{\sigma^2}+\frac{2bf}{\sigma^2}-2b\mu^3-2b\mu+\frac{f^4}{\sigma^4}-\frac{2f^2\mu^2}{\sigma^2}-\frac{2f^2}{\sigma^2}+\mu^4+2\mu^2+1 ] \nonumber
\end{align}
Recalling:
\begin{align}
    \mathbb{E}(f) &= \mu \\
    \mathbb{E}(f^2) &= \sigma^2 + \mu \\
    \mathbb{E}(f^3) &=  \mu^3 + 3\mu \sigma^2\\
    \mathbb{E}(f^4) &= \mu^4 + 6 \mu^2 \sigma^2 + 3 \sigma^4
\end{align}

We have:
\begin{dmath}
    \mathbb{C}\text{ov}(X,Y) =  \left(a^2 \left(\sigma^2-1\right)^2 (b-\mu)^2-2 a \left(b^2 \mu \left(\sigma^2-1\right)^2-2 b \left(\mu^2 \left(\sigma^2-1\right)^2+\sigma^2\right)+\mu ^3 \left(\sigma ^2-1\right)^2+2 \mu  \sigma ^2\right) +b^2 \mu^2
    \left(\sigma ^2-1\right)^2-2 b \left(\mu ^3 \left(\sigma ^2-1\right)^2+2 \mu 
   \sigma ^2\right)+\mu ^4 \sigma ^4-2 \mu ^4 \sigma ^2+\mu ^4+4 \mu ^2 \sigma ^2+2
   \sigma ^4\right) \frac{1}{\sigma^4}
\end{dmath}
